# Supplementary material for: Guiding-Based Importance Sampling for Walk on Stars
Source: arXiv:2410.18944 source file (2025-05-01)
Supplement: Supplementary file 1 [file suppl.pdf]

# Supplementary Material for Guiding-Based Importance Sampling for Walk on Stars


TIANYU HUANG, School of Software and BNRist, Tsinghua University, China
JINGWANG LING, School of Software and BNRist, Tsinghua University, China
SHUANG ZHAO, University of California Irvine, United States of America
FENG XU*, School of Software and BNRist, Tsinghua University, China



**ACM Reference Format:**
Tianyu Huang, Jingwang Ling, Shuang Zhao, and Feng Xu. 2025. Supplementary Material for Guiding-Based Importance Sampling for Walk on Stars. In *Special Interest Group on Computer Graphics and Interactive Techniques Conference Conference Papers (SIGGRAPH Conference Papers '25), August 10–14, 2025, Vancouver, BC, Canada.* ACM, New York, NY, USA, 3 pages. https://doi.org/10.1145/3721238.3730593


## A von Mises-Fisher (vMF) Distribution

Below, we present the 2D and 3D formulations of the vMF distribution:

$$v^{2\mathrm{D}}(v \mid \mu, \kappa) = \frac{\exp(\kappa \mu^{\mathrm{T}} v)}{2\pi I_0(\kappa)},$$

$$v^{3\mathrm{D}}(v \mid \mu, \kappa) = \frac{\kappa}{4\pi \sinh \kappa} \exp(\kappa \mu^{\mathrm{T}} v).$$

## B Derivation of the Reparametrization of the Walk on Stars Estimator

The Boundary Integral Formulation [Sawhney et al. 2023] for the Poisson equation is given as:

$$\alpha(x)u(x) = \int_{\partial \mathrm{St}(x,r)} P^B(x,z)u(z)\mathrm{d}z - \int_{\partial \mathrm{St}_N(x,r)} G^B(x,z)h(z)\,\mathrm{d}z + \int_{\mathrm{St}(x,r)} G^B(x,y)f(y)\,\mathrm{d}y.$$

The first term, which is:

$$u_1(x) = \frac{1}{\alpha(x)} \int_{\partial \mathrm{St}(x,r)} P^B(x,z)u(z)\mathrm{d}z,$$

corresponds to the recursive Monte Carlo integration in the WoSt estimator. Consider the 3D case. Substituting

$$P^{\mathrm{B,3D}}(x,z) = \frac{n_z \cdot (z-x)}{4\pi \|z-x\|^3}$$

into $u_1(x)$, we obtain:

$$u_1(x) = \frac{1}{\alpha(x)} \int_{\partial \mathrm{St}(x,r)} \frac{n_z \cdot (z-x)}{4\pi \|z-x\|^3} u(z)\mathrm{d}z.$$

We perform a change of variables by letting $\frac{z-x}{\|z-x\|} = v$ and setting $\|z-x\| = r$, which gives:

$$u_1(x) = \frac{1}{\|\mathbb{S}^2\| \alpha(x)} \int_{\partial \mathrm{St}(x,r)} u(v;x) \frac{(n_z \cdot v)\mathrm{d}z}{r^2} = \frac{1}{\|\mathbb{S}^2\| \alpha(x)} \int_{\mathbb{S}^2} u(v;x)\mathrm{d}v.$$

Its corresponding single-sample Monte Carlo estimator is:

$$\langle u_1(x) \rangle = \frac{\langle u(v;x) \rangle}{\|\mathbb{S}^2\|\, \alpha(x)\, p^{\mathbb{S}^2}(v \mid x)}.$$

The 2D case follows similarly. We note that a similar derivation [Veach 1998] also exists in the Monte Carlo rendering domain.

## C Comparison with Existing Variance Reduction Methods

As described in Section 6, we have chosen to compare our method only with the original WoSt in the main text of this paper. This decision is based on several factors: our approach is not a replacement or refinement of existing methods, but orthogonal to them; moreover, our method and existing approaches are implemented on different systems, making a fair comparison challenging. These challenges have also been noted by Bakbouk and Peers [2023, Section 10]. Nevertheless, to demonstrate the distinguishing features of our method, in this section, we conduct a few comparison with selected existing methods using metrics that are as comparable as possible.

### C.1 Neural Caches

*Neural caches* [Li et al. 2023] is another variance reduction method for WoSt that leverages a neural field. However, unlike our approach, which uses a neural field to encode a space-conditioned guiding distribution, neural caches directly employs a neural field to cache the solution value field in space. Unlike our online training approach, where training and inference occur progressively and simultaneously, neural caches explicitly separates the solving process into distinct training and inference stages. This distinction makes cross-system comparisons challenging. Therefore, we decide to pretrain


*Corresponding author.

Authors' Contact Information: Tianyu Huang, School of Software and BNRist, Tsinghua University, Beijing, China, huang-ty21@mails.tsinghua.edu.cn; Jingwang Ling, School of Software and BNRist, Tsinghua University, Beijing, China, lingjw20@mails.tsinghua.edu.cn; Shuang Zhao, University of California Irvine, Irvine, United States of America, shz@ics.uci.edu; Feng Xu, School of Software and BNRist, Tsinghua University, Beijing, China, xufeng2003@gmail.com.



*SIGGRAPH Conference Papers '25, August 10–14, 2025, Vancouver, BC, Canada*
© 2025 Copyright held by the owner/author(s).
This is the author's version of the work. It is posted here for your personal use. Not for redistribution. The definitive Version of Record was published in *Special Interest Group on Computer Graphics and Interactive Techniques Conference Conference Papers (SIGGRAPH Conference Papers '25), August 10–14, 2025, Vancouver, BC, Canada*, https://doi.org/10.1145/3721238.3730593.

a checkpoint and then use the inference stage of neural caches to perform a comparison with our method under equal wpp condition.

Since the authors of neural caches have not released their code, we reproduce their work using PyTorch [Paszke et al. 2019]. We train and evaluate their approach on a 2D Laplace problem following the exact methodology described in their paper. Consistent with the design of their experiments in the original paper, we set the hyperparameter $m = 1$ or $m = 5$, meaning that performing 1 or 5 steps, *resp.*, before querying the neural field cache. The experimental results are presented in Fig. 1, where we illustrate the problem setting, the convergence plots of different methods, and a qualitative and quantitative comparison of relMSE at 256 wpp and 2048 wpp.

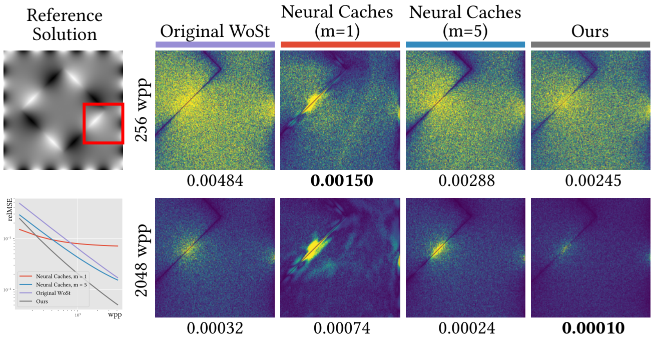


Fig. 1. Comparison with neural caches [Li et al. 2023] in a 2D problem.

The convergence plot aligns with the results reported by Li et al. [2023, Section 7.3 and 7.4]. The experiment demonstrates that pre-trained neural caches can reduce variance at low sample counts. However, due to the expressive limitations of PINNs, the solution field cached by neural caches exhibits bias, which becomes increasingly evident at higher sample counts, eventually allowing the original WoSt to outperform it. Our method does not introduce additional bias, and by significantly improving the convergence rate of WoSt, greatly narrows the advantage range of neural caches. As shown in this experiment, our approach surpasses neural caches ($m = 1$) at approximately 100–200 wpp and is always better than neural caches ($m = 5$).

### C.2 Reverse Walk Splatting

*Reverse walk splatting (RWS)* [Qi et al. 2022] adopts a strategy opposite to those of the original WoSt and ours, performing random walks from boundaries and source rather than from the evaluation points. This approach demonstrates strong performance in 2D scenarios, as the sampling space of boundaries and source is often smaller than or comparable to that of the evaluation grid, and it is easy for reverse walks to fall on the evaluation grid. However, in 3D scenarios, particularly when solving on slices [Sawhney and Crane 2020, Section 5.2], the sampling space of boundaries and source may exceed that of the evaluation grid. Besides, in 3D, the contributions from reverse walks are less likely to fall on the evaluation grid, leading to overhead and performance degradation. To illustrate this, we design a simple experiment, as shown on the far-left side of Fig. 2.

RWS does not have the concept of wpp. Therefore, we manage to achieve fairness by adjusting the number of sampling points originating from boundaries and source. In our experiment, we apply the following method to match the sample count: for RWS, we set the number of sample points on the Dirichlet boundaries to $256 \times 256 \times 1024$. Since there are no Neumann boundaries or source in this problem, we set the number of their sample points to 0. For the original WoSt and our method, we perform 1024 samples on a $256 \times 256$ evaluation grid. The experimental results are shown in Fig. 2.

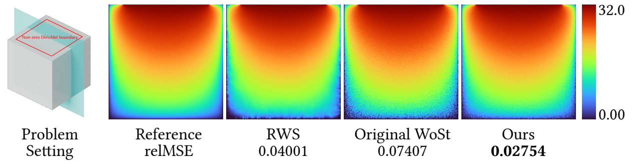


Fig. 2. Comparison with reverse walk splatting (RWS) [Qi et al. 2022] in a 3D problem. Although RWS produces smooth results, correlation artifacts are observed. In this experiment, the quantitative metric for RWS outperforms the original WoSt, but is weaker than ours.

The experimental results of this problem align with our previous analysis, demonstrating that in 3D scenarios involving solving on slices where the evaluation grid has a relatively small sampling space, our method outperforms RWS both qualitatively and quantitatively under the same number of samples. Additionally, our approach avoids noticeable correlation artifacts. Our method retains the advantages of the original WoSt by not introducing unnecessary sampling.

## D Detailed Configurations of Our Neural Field

In this section, we present the detailed configuration of our neural field. Tab. 1 lists the configuration parameters for the multi-resolution feature grid, Tab. 2 presents the parameters for the multi-layer perceptron (MLP), and Tab. 3 specifies the optimizer settings. We acknowledge that an optimal set of parameters may vary depending on the dimensionality and nature of the problem. However, to demonstrate the general applicability of our approach, we have employed the same set of parameters across all experiments.

Table 1. Encoding Parameters. The Per Level Scale is utilized to generate the sequence of $D_l^d$. For instance, under this configuration, $D_8^d = \lfloor D_1^d \times 1.405^{(8-1)} \rfloor = 86$.

| **Parameter** | **Value** |
|---|---|
| Base Resolution $D_1^d$ | 8 |
| Interpolation | `Linear` |
| Features per Level $F$ | 4 |
| Number of Levels $L$ | 8 |
| Type | `DenseGrid` |
| Per Level Scale | 1.405 |

Table 2. MLP Parameters. FullyFusedMLP is a high-performance MLP implementation provided by *tiny-cuda-nn* [Müller 2021]. The Activation here does not apply to the last layer, as the last layer employs our custom-defined normalization mappings.

| Parameter | Value |
|---|---|
| Activation | ReLU |
| Hidden Layers | 3 |
| Neurons | 64 |
| Type | FullyFusedMLP |

Table 3. Optimizer Parameters.

| Parameter | Value |
|---|---|
| **Optimizer** | |
| Decay | 0.95 |
| Type | Ema |
| **Nested Optimizer (Adam)** | |
| AdaBound | False |
| Beta1 | 0.9 |
| Beta2 | 0.99 |
| Epsilon | 1.0e-15 |
| L2 Regularization | 1.0e-6 |
| Learning Rate | 0.008 |
| Type | Adam |

## E Raw Quantitative Data of Experiments

In this section, we present the complete quantitative experimental results (at 1024 wpp) corresponding to the experiments in the main text. We report both the relative MSE and the runtime. Following the order of the original paper, the results are shown in Tab. 4, Tab. 5, Tab. 6, and Tab. 7.

Table 4. Raw quantitative data of the 3D geometry experiments at 1024 wpp.

| | relative MSE | | Runtime (s) | |
|---|---|---|---|---|
| Problem | Original WoSt | Ours | Original WoSt | Ours |
| Bob | 0.003992 | 0.000981 | 268.93 | 305.24 |
| Bunny | 0.015115 | 0.005643 | 868.52 | 1119.8 |
| Dragon | 0.003789 | 0.000878 | 461.55 | 523.27 |
| Gear | 0.001528 | 0.000720 | 555.55 | 609.04 |
| Bottle | 0.004593 | 0.002743 | 712.34 | 879.42 |
| Spot | 8.275137 | 4.157117 | 105.67 | 129.14 |

Table 5. Raw quantitative data of the 2D diffusion curve experiments at 1024 wpp.

| | relative MSE | | Runtime (s) | |
|---|---|---|---|---|
| Problem | Original WoSt | Ours | Original WoSt | Ours |
| Fille | 0.005229 | 0.002084 | 242.86 | 280.68 |
| Ladybug | $7.026 \times 10^{-5}$ | $4.506 \times 10^{-5}$ | 207.33 | 225.11 |

Table 6. Raw quantitative data of the training batch size evaluation experiments at 1024 wpp.

| | relative MSE | | | | Runtime (s) | | | |
|---|---|---|---|---|---|---|---|---|
| Problem | 64 | 128 | 256 | 512 | 64 | 128 | 256 | 512 |
| Bob | 0.001060 | 0.001023 | 0.000971 | 0.000961 | 293.65 | 295.56 | 298.22 | 306.14 |
| Bunny | 0.005725 | 0.005612 | 0.005563 | 0.005615 | 1087.3 | 1094.5 | 1105.9 | 1125.6 |
| Dragon | 0.001185 | 0.000985 | 0.000934 | 0.000889 | 510.56 | 513.19 | 517.41 | 525.17 |
| Gear | 0.000790 | 0.000720 | 0.000717 | 0.000702 | 597.70 | 601.78 | 602.69 | 607.00 |
| Bottle | 0.002817 | 0.002761 | 0.002767 | 0.002747 | 867.83 | 870.67 | 874.82 | 883.10 |
| Fille | 0.002243 | 0.002130 | 0.002114 | 0.002060 | 264.80 | 268.20 | 275.12 | 284.71 |

Table 7. Raw quantitative data of the number of vMF components evaluation experiments at 1024 wpp.

| | relative MSE | | | Runtime (s) | | |
|---|---|---|---|---|---|---|
| Problem | 4 | 8 | 16 | 4 | 8 | 16 |
| Bob | 0.001107 | 0.000957 | 0.000949 | 294.73 | 298.14 | 302.18 |
| Bunny | 0.005731 | 0.005559 | 0.005576 | 1103.5 | 1111.4 | 1115.5 |
| Dragon | 0.001185 | 0.000887 | 0.000894 | 514.68 | 517.39 | 523.06 |
| Gear | 0.000730 | 0.000703 | 0.000703 | 604.77 | 602.70 | 599.60 |
| Bottle | 0.002824 | 0.002732 | 0.002691 | 871.54 | 876.53 | 874.91 |
| Fille | 0.002096 | 0.002090 | 0.002084 | 298.60 | 269.08 | 274.85 |

## References

Ghada Bakbouk and Pieter Peers. 2023. Mean Value Caching for Walk on Spheres. In *Eurographics Symposium on Rendering*, Tobias Ritschel and Andrea Weidlich (Eds.). The Eurographics Association. https://doi.org/10.2312/sr.20231120

Zilu Li, Guandao Yang, Xi Deng, Christopher De Sa, Bharath Hariharan, and Steve Marschner. 2023. Neural Caches for Monte Carlo Partial Differential Equation Solvers. In *SIGGRAPH Asia 2023 Conference Papers* (Sydney, NSW, Australia) *(SA '23)*. Association for Computing Machinery, New York, NY, USA, Article 34, 10 pages. https://doi.org/10.1145/3610548.3618141

Thomas Müller. 2021. *tiny-cuda-nn*. https://github.com/NVlabs/tiny-cuda-nn

Adam Paszke, Sam Gross, Francisco Massa, Adam Lerer, James Bradbury, Gregory Chanan, Trevor Killeen, Zeming Lin, Natalia Gimelshein, Luca Antiga, Alban Desmaison, Andreas Köpf, Edward Yang, Zach DeVito, Martin Raison, Alykhan Tejani, Sasank Chilamkurthy, Benoit Steiner, Lu Fang, Junjie Bai, and Soumith Chintala. 2019. *PyTorch: an imperative style, high-performance deep learning library.* Curran Associates Inc., Red Hook, NY, USA.

Yang Qi, Dario Seyb, Benedikt Bitterli, and Wojciech Jarosz. 2022. A bidirectional formulation for Walk on Spheres. *Computer Graphics Forum (Proceedings of EGSR)* 41, 4 (July 2022). https://doi.org/10/jgzr

Rohan Sawhney and Keenan Crane. 2020. Monte Carlo Geometry Processing: A Grid-Free Approach to PDE-Based Methods on Volumetric Domains. *ACM Trans. Graph.* 39, 4 (2020).

Rohan Sawhney, Bailey Miller, Ioannis Gkioulekas, and Keenan Crane. 2023. Walk on Stars: A Grid-Free Monte Carlo Method for PDEs with Neumann Boundary Conditions. *ACM Trans. Graph.* 42, 4 (2023).

Eric Veach. 1998. *Robust Monte Carlo methods for light transport simulation.* Stanford University.
